# Supplementary material for: From Physical to Cyber: Escalating Protection for Personalized Auto Insurance
Source: arXiv:1609.02234 source file (2017-05-23)
Supplement: Supplementary file 1 [file appendix.tex]

\appendix

\section{Insurer's Web Interface}
\label{app:anomaly}

Insurers provide web interfaces for their customers. Through web interfaces,
policyholders can review when they use their vehicle, how far they drive and how
hard they brake etc. Figure~\ref{fig:abnormaldetection} shows the web interface
of Progressive which illustrates an anomalous trip.

\begin{figure}[h]
\centering
  \includegraphics[width=0.9\columnwidth]{./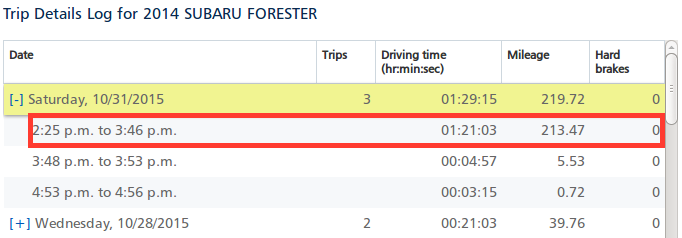}
  \caption{An evidence showing the absence of anomaly detection on Progressive.}
  \label{fig:abnormaldetection}
\end{figure}

\section{Attack}
\label{app:attack}

\begin{figure}[h]
\centering
  \includegraphics[width=0.9\columnwidth]{./figures/schema.pdf}
  \caption{The components resided in the man-in-the-middle box.}
  \label{fig:smootherschematic}
\end{figure}

\begin{figure}[h]
\centering
  \includegraphics[width=0.9\columnwidth]{./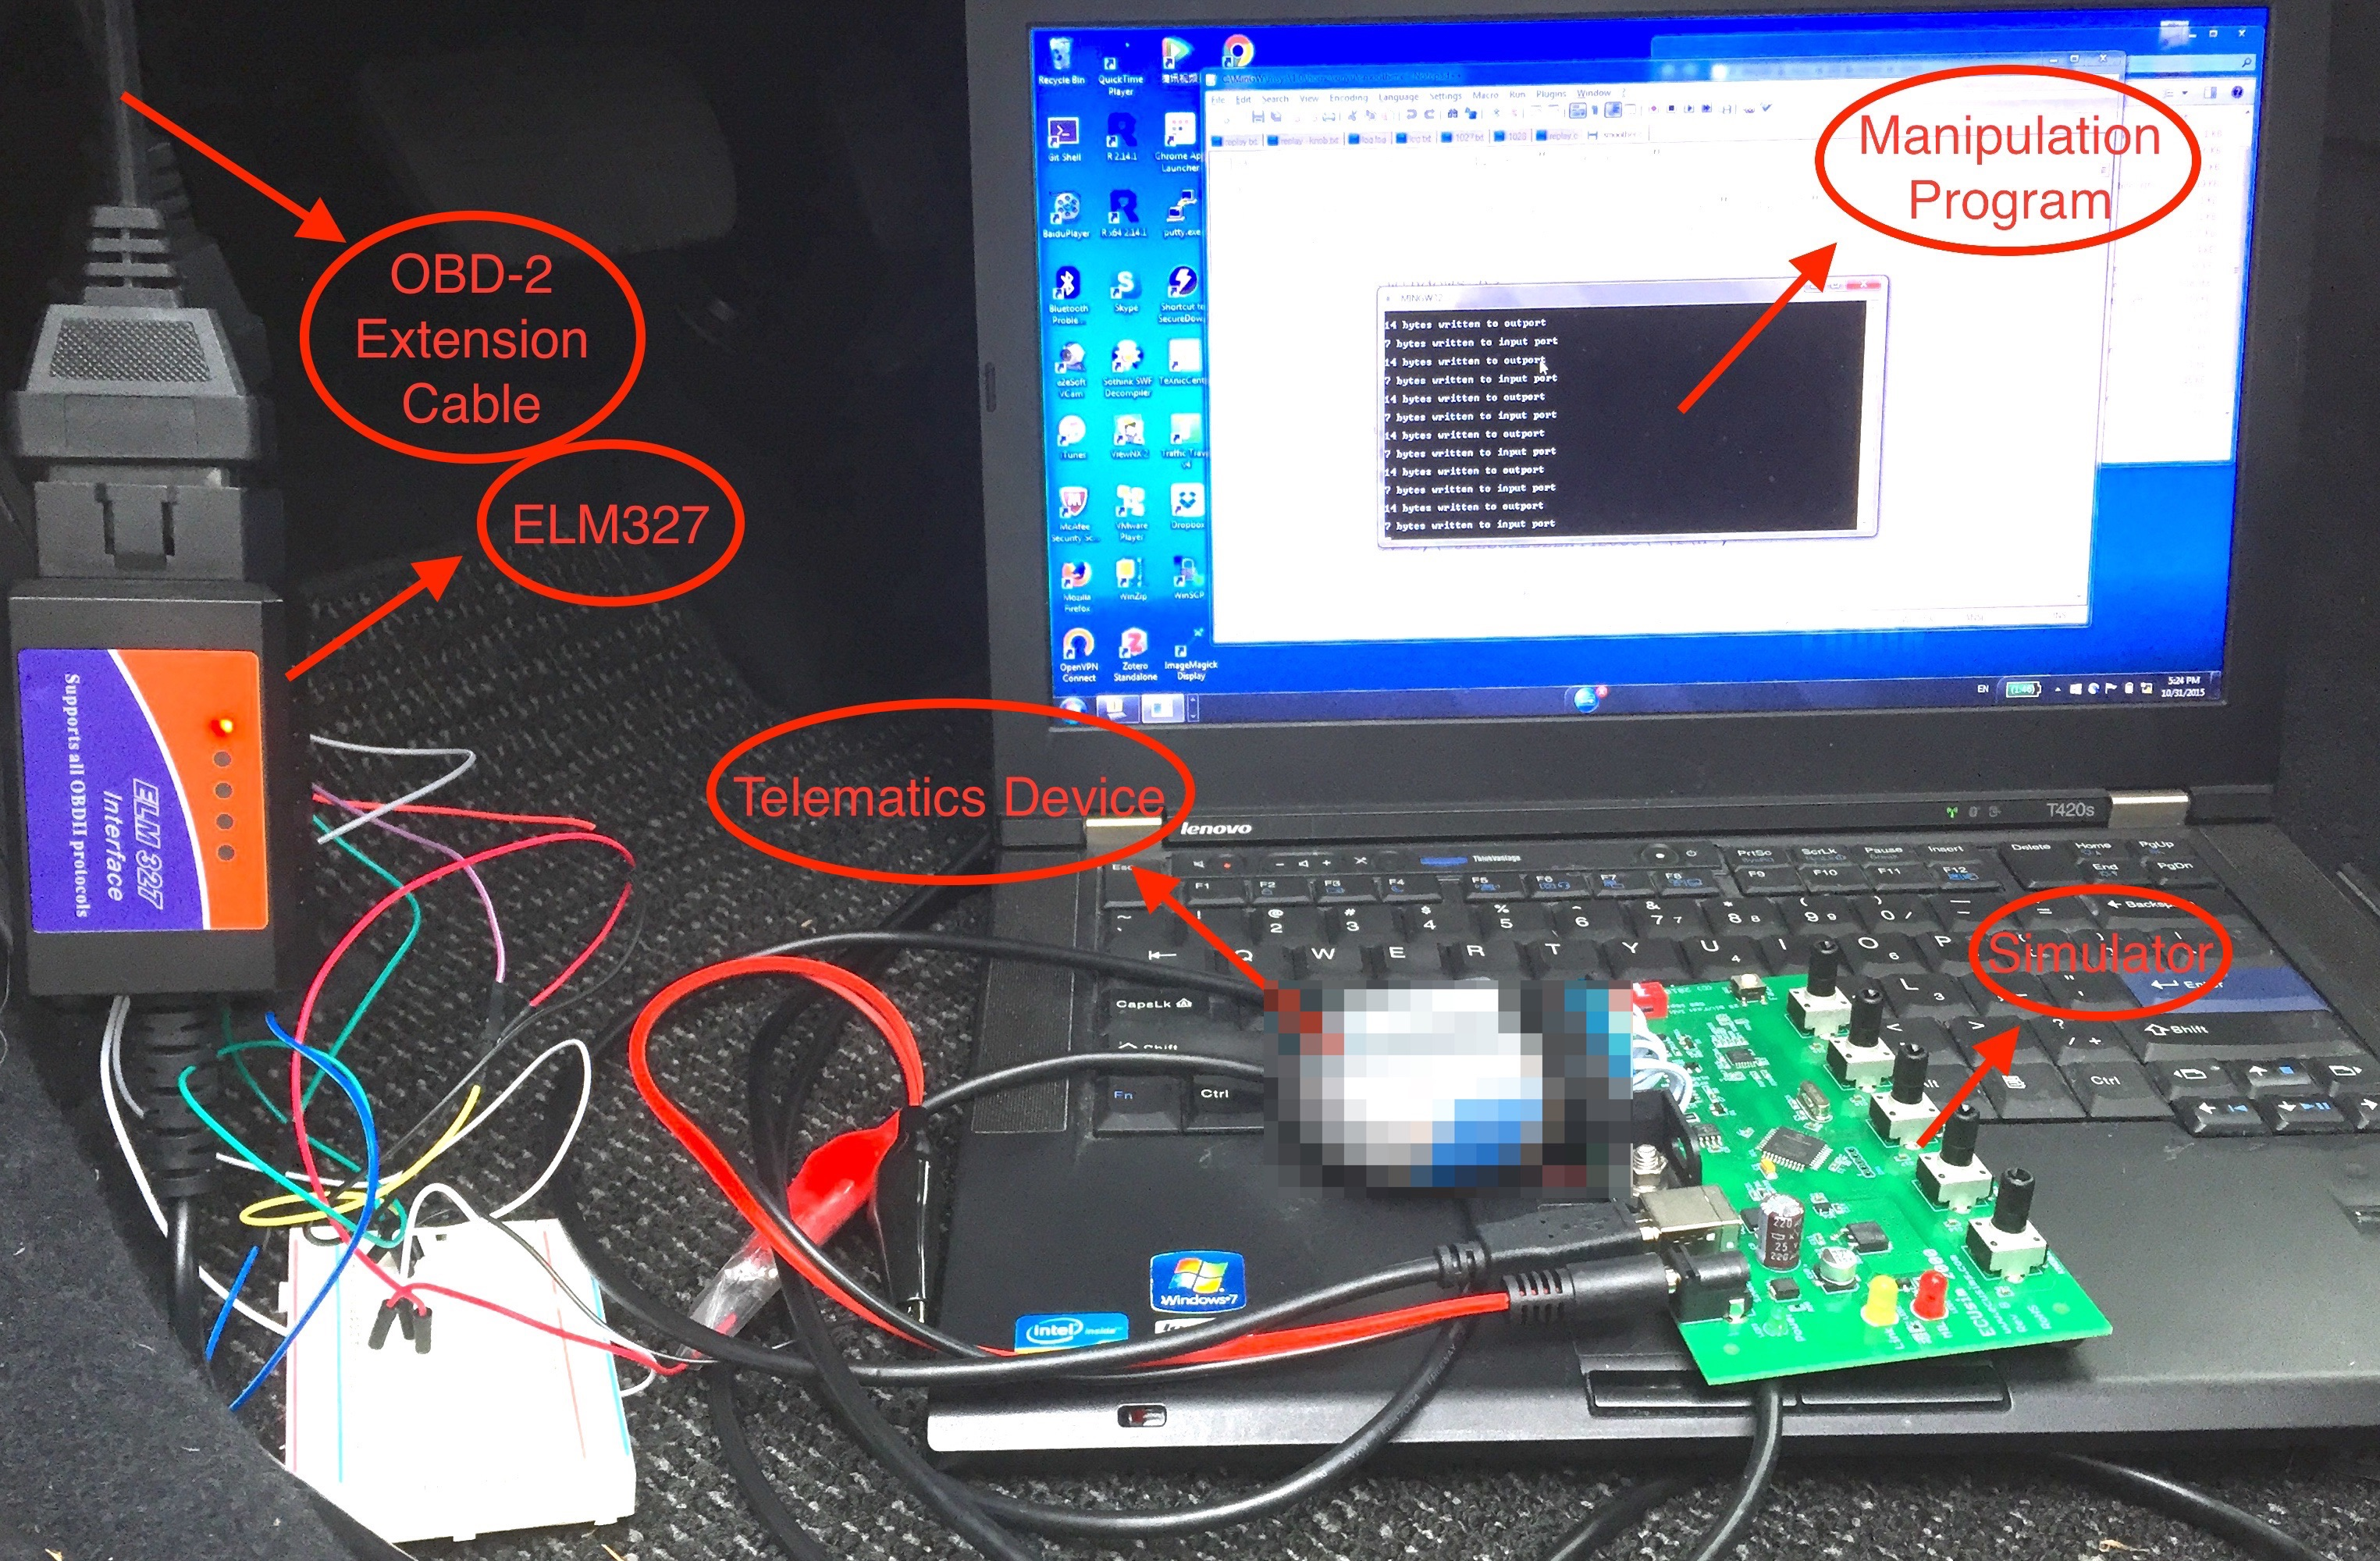}
  \caption{The man-in-the-middle box that bridges a car's OBD-2 port and  a Progressive's Snapshot device.}
  \label{fig:inthecar}
\end{figure}

We developed a box that manipulates speed readings when the speed readings
indicate dangerous driving activities. Figure~\ref{fig:smootherschematic}
and~\ref{fig:inthecar} show how the box is assembled logically and physically,
respectively.
